# Supplementary material for: Generating Entangled Microwave Radiation Over Two Transmission Lines
Source: arXiv:1204.0732 ancillary file (2012-10-31)
Supplement: Supplementary file 1 [file Flurin-SupInfo.pdf]

# Supplementary information: Producing and measuring entanglement between two beams of microwave light

E. Flurin,<sup>1</sup> N. Roch,<sup>1</sup> F. Mallet,<sup>1</sup> M. H. Devoret,<sup>2,1,3</sup> and B. Huard<sup>1,\*</sup>

<sup>1</sup>*Laboratoire Pierre Aigrain, Ecole Normale Supérieure,*

*CNRS (UMR 8551), Université P. et M. Curie,*

*Université D. Diderot 24, rue Lhomond, 75231 Paris Cedex 05, France*

<sup>2</sup>*Collège de France, 11 Place Marcelin Berthelot, F-75231 Paris Cedex 05, France*

<sup>3</sup>*Department of Applied Physics, Yale University, PO Box 208284, New Haven, CT 06520-8284*

## MEASUREMENT SETUP

In this section, we fully describe the measurement setup at every temperature stage (Fig. 1). Two important features, not described in the main text, are presented: the noise calibration circuit and the pump leakage compensation circuit.

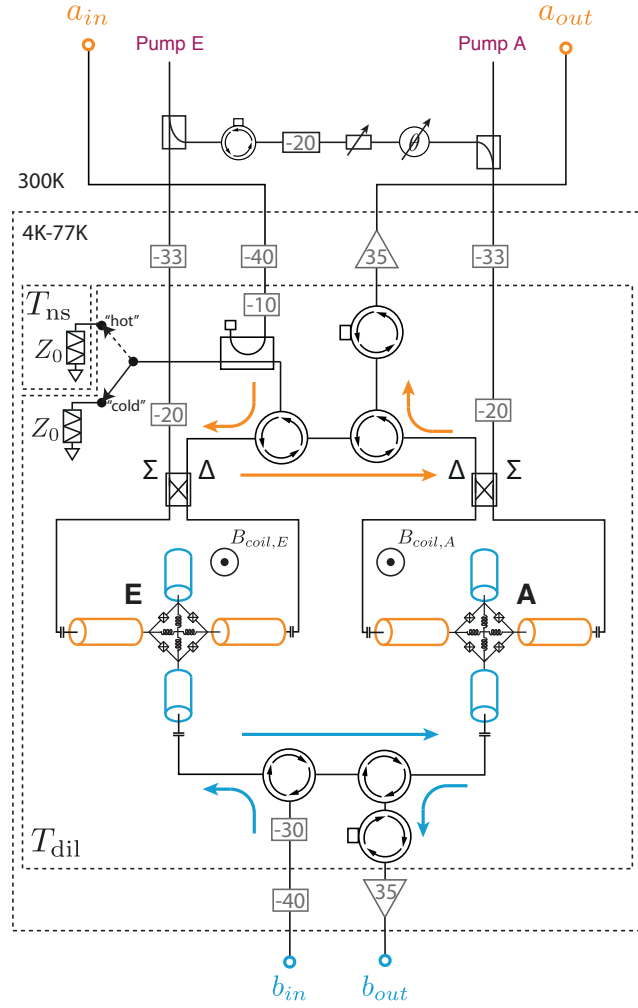

FIG. 1: Detailed measurement setup. The gray rectangles stand for microwave attenuators. The gray triangles are HEMT amplifiers. The two Josephson mixers (labeled E and A) are embedded in the same Cryoperm magnetic shield (not shown on the figure)

### Calibration circuit

A microwave switch was inserted at the input of the setup on  $a_{in,E}$  through a directional coupler (see Fig. 1). In the "cold" position, the switch is fed by a cold  $50\ \Omega$  load at dilution refrigerator temperature  $T_{dil}$ . In the "hot" position, the switch is fed by a  $50\ \Omega$  load with variable temperature  $T_{ns}$ . It is placed on a copper plate which is only weakly thermally anchored to the mixing chamber stage through a thin stainless steel tubing 4 mm long and  $2\text{ mm}^2$  in cross-section. Temperature  $T_{ns}$  can be finely tuned using a heater resistor and calibrated  $\text{RuO}_2$  thermometer fixed to the copper plate.  $T_{ns}$  can be varied from 90 mK to 900 mK within a few tens of minutes without any effect on the temperature  $T_{dil}$  of the mixing chamber to which the Josephson mixers are thermally anchored. Reaching lower temperatures  $T_{ns}$  than 90 mK is possible but requires of the order of 50 hours for thermalization. Hence the use of a microwave switch to access almost instantaneously the base temperatures  $T_{ns} = T_{dil}$ .

### Pump leakage compensation circuit

Instead of using a single split microwave source for pumping both mixers, it is more practical to use two synchronized sources (Fig. 1). The phase difference between the two pumps is then increased by slightly detuning one source with respect to the other. For the measurements presented in the main text, the detuning is  $\delta\omega/2\pi = 0.3\text{ Hz}$ . The phase difference is then given by  $\Delta\varphi = \delta\omega t$ .

The frequency tunability of the mixers offer a way to remove any small contribution to the measured interferences coming from a direct beating between leaking pump signals. Such parasitic contributions appear, for instance, if the entangler pump signal leaks towards the analyzer pump port, and effective pump amplitude feeding the analyzer reads

$$\mathcal{A}_P(t) = \mathcal{A}_{P_A}[\sin(\omega_P t) + \epsilon \sin(\omega_P t + \delta\omega t + \theta)] \quad (1)$$

where  $\omega_P = 14.390\text{ GHz}$  is the analyzer pump frequency,  $\theta$  is a fixed phase offset and  $\epsilon \ll 1$  is the leakage fraction from the entangler pump to the analyzer pump. This translates into a modulating value of the squeezing parameter

$$r_A \propto 1 + \epsilon \cos(\delta\omega t + \theta). \quad (2)$$

Conveniently, by flux detuning the entangler to a working point where it does not present any non-linearity (top the arches on Fig. 4a, see Ref. [1]), all the observed modulation in the transmission comes from parasitic leaks. We could observe a tiny modulation corresponding to  $\epsilon \lesssim 10^{-2}$ . Reversing the roles of both mixers, we could determine that the leak from the analyzer pump towards the entangler was at least 2 orders of magnitude weaker.

In order to get rid of this leakage, we added a compensation circuit (see Fig. 1) at room temperature, consisting of a variable attenuator and a variable phase shifter. To get the best sensitivity, we tuned these variable components while operating the analyzer close to its parametric oscillation threshold (gain  $> 25\text{ dB}$ ). Note that, without this compensation, the interference fringes shown in the main text would be slightly asymmetric due to the fact that  $\theta \neq 0, \pi$  in the experiment.

### NOISE MEASUREMENT PROCEDURE

To reduce drifts and uncertainties during the measurement, we used the following automatized procedure. The final  $a$  channel output is split, and sent to both a 4-port Vector Network Analyzer (VNA) and a Power Spectrum Analyzer (PSA). The  $b$  output is sent to the VNA also. We can precisely compensate for drifts in the gain of both the entangler and analyzer (or equivalently, the value of  $r_A$  and  $r_E$ ), thanks to a feedback scheme on the value of each pump power. For each couple of chosen gains  $G_E$  for the entangler and  $G_A$  for the analyzer, the following sequential procedure is performed in a couple of minutes only.

| operation                                   | entangler | analyzer | comments                      |
|---------------------------------------------|-----------|----------|-------------------------------|
| measure transmission reference              | Off       | Off      | VNA                           |
| measure noise power $S_{\text{off}}$        | Off       | Off      | PSA, RBW : 510 kHz            |
| feedback on $P_E$ to reach $G_E$            | On        | Off      | VNA, precision: $\pm 0.05$ dB |
| measure noise power $S_E$                   | On        | Off      | PSA, RBW : 510 kHz            |
| feedback on $P_A$ to reach $G_A$            | Off       | On       | VNA, precision: $\pm 0.05$ dB |
| measure noise power $S_A$                   | Off       | On       | PSA, RBW : 510 kHz            |
| measure transmission: $t_{a \rightarrow a}$ | On        | On       | VNA                           |
| measure transmission: $t_{a \rightarrow b}$ | On        | On       | VNA                           |
| measure noise power $S_a(\Delta\varphi)$    | On        | On       | PSA, RBW : 510 kHz            |

## NOISE CALIBRATION

### Converting measured spectral density into quanta of output noise

This section shows how to relate the measured noise spectral density  $S_a(f_a)$  at the end of the measurement setup (Fig. 4a in the main text) to the variance of the field operator at the output of the analyzer ( $\Delta a_{out,A}^2$ ). As shown in the main text, the scattering matrix of the two mixers in series can be measured directly (Fig. 3 in the main text). For each values of the pump powers, it is thus possible to determine the values of the squeezing parameters  $r_E$  and  $r_A$ . As shown in Fig. 3, all the data can be explained by a unique ratio  $(1 - \beta)/(1 - \alpha) = 0.945$  between the unbalanced losses on both arms connecting the mixers. Four parameters remain to be determined in order to fully calibrate the noise measurements. First, the low noise amplifier followed by square law detector at the output  $a_{out,A}$  adds a noise offset  $S_{\text{LNA}}$  and amplifies the noise by a gain  $G_{\text{LNA}}$ . Second, the absolute losses  $\alpha$  and  $\beta$  are unknown. Finally, the system noise added by the mixers needs to be determined.

In what follows, we will assume that the Josephson mixers are ideal, in the sense that they do not add any spurious noise coming from uncontrolled channels. However, insertion losses (like  $\alpha$  and  $\beta$ ) can degrade the system measurement efficiency of these amplifiers. The losses between the load noise source and the mixer port  $a_{in,E}$  are modeled by a beam splitter with transmission  $\gamma$  (a fraction  $1 - \gamma$  of the power coming from the noise source reaches the entangler). The system noise is quantified by  $\gamma$ , since this model is equivalent to considering perfect transmission between the noise source and the mixer with an added noise of  $\gamma/(2 - 2\gamma)$  quanta referred to the input.

The calibration involves noise measurements in three configurations:  $S_{\text{off}}$  when analyzer and entangler are turned off ( $r_A = r_E = 0$ ),  $S_E$  when only the entangler is turned on ( $r_A = 0$ ) and  $S_A$  when only the analyzer is turned on ( $r_E = 0$ ). In order to give simple expressions for these three noise powers, we introduce the attenuations  $\bar{\alpha} = 1 - \alpha$ ,  $\bar{\gamma} = 1 - \gamma$ , and the noise spectra  $S_{\text{dil},a} = \langle (\Delta a)^2 \rangle_{T_{\text{dil}}} = \frac{1}{2} \coth(hf_a/2k_B T_{\text{dil}})$ ,  $S_{\text{dil},b} = \langle (\Delta b)^2 \rangle_{T_{\text{dil}}} = \frac{1}{2} \coth(hf_b/2k_B T_{\text{dil}})$ , and  $S_{\text{ns}} = \langle (\Delta a)^2 \rangle_{T_{\text{ns}}} = \frac{1}{2} \coth(hf_a/2k_B T_{\text{ns}})$ , where  $\langle \cdot \rangle_T$  denotes the average of an operator in the thermal state of temperature  $T$ .

During the experiment described in the main text, the switch is in the cold load position so that  $S_{\text{ns}} = S_{\text{dil},a}$  and one can determine directly the noise at the analyzer output from the measured noise power  $S_a$ . Indeed, since  $S_a = S_{\text{LNA}} + G_{\text{LNA}} hf_a (\Delta a_{out,A})^2$ , the output noise is

$$(\Delta a_{out,A})^2 = \frac{S_a - S_{\text{off}}}{G_{\text{LNA}} hf_a} + S_{\text{dil},a}. \quad (3)$$

In practice, the noise added by the measurement setup  $S_{\text{LNA}}$  drifts slowly with time so that all quantities are rapidly measured one after the other and subtracted (see table above).

### Calibration of relevant parameters using a thermal noise source

It is straightforward to show that

$$S_{\text{off}} = S_{\text{LNA}} + G_{\text{LNA}} hf_a [\bar{\alpha} \bar{\gamma} S_{\text{ns}} + (1 - \bar{\alpha} \bar{\gamma}) S_{\text{dil},a}] \quad (4)$$

$$S_E = S_{\text{LNA}} + G_{\text{LNA}} hf_a [\bar{\alpha} \bar{\gamma} S_{\text{ns}} \cosh^2 r_E + \bar{\alpha} (1 - \bar{\gamma}) S_{\text{dil},a} \cosh^2 r_E + \bar{\alpha} S_{\text{dil},b} \sinh^2 r_E + (1 - \bar{\alpha}) S_{\text{dil},a}] \quad (5)$$

$$S_A = S_{\text{LNA}} + G_{\text{LNA}} hf_a [\bar{\alpha} \bar{\gamma} S_{\text{ns}} \cosh^2 r_A + (1 - \bar{\alpha} \bar{\gamma}) S_{\text{dil},a} \cosh^2 r_A + S_{\text{dil},b} \sinh^2 r_A]. \quad (6)$$

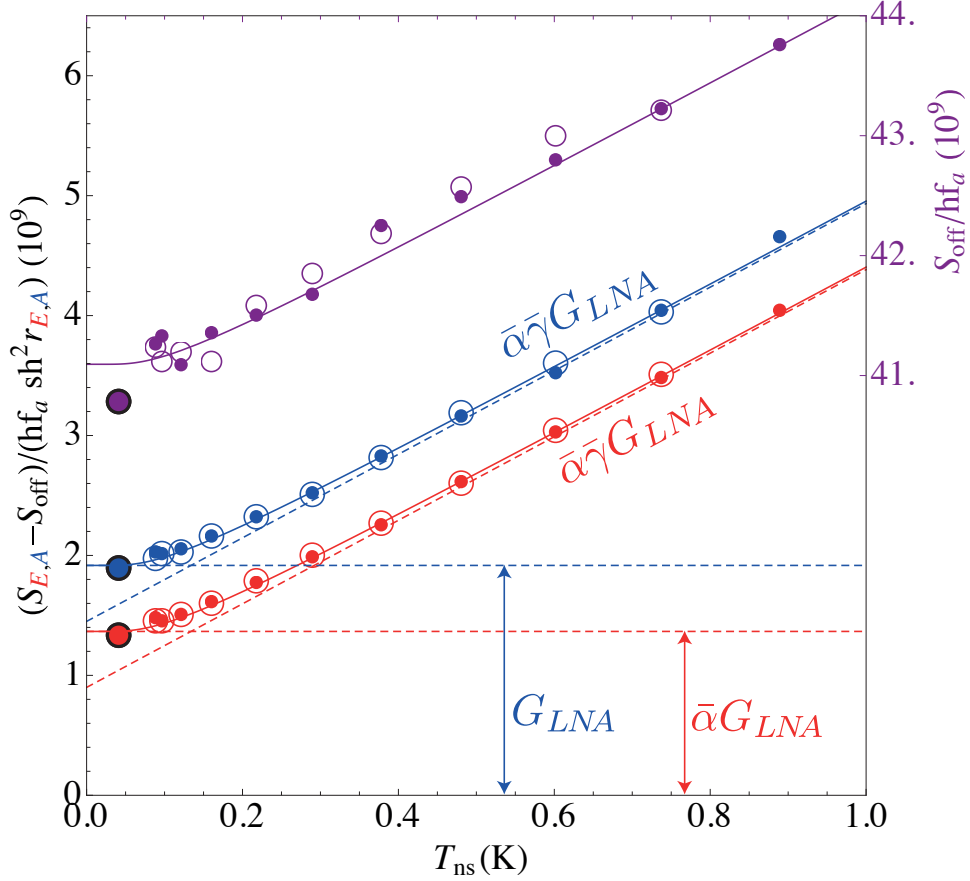

FIG. 2: Red dots: difference between measured spectral densities  $S_E$  and  $S_{\text{off}}$  normalized by  $hf_a \sinh^2 r_E$  as a function of noise source temperature  $T_{\text{ns}}$ . These values are averaged over 6 entangler gains from 3 to 100. Filled circles correspond to the measurements made with increasing temperature from dot to dot. Empty circles correspond to decreasing temperatures. Blue dots: same measurements for the analyzer averaged over 3 analyzer gains from 10 to 100. Purple dots: level of noise  $S_{\text{off}}$  when both mixers are not pumped. Note that the scale is not divided by  $\sinh^2 r$ . Dashed lines: The slope of both red and blue curves at large temperature and the offset of these curves lead to independent determination of the three free parameters to calibrate. Lines: best fit of the data using Eqs. (7,8) with  $\alpha = 0.33 \pm 0.05$ ,  $\gamma = 0.28 \pm 0.11$  and  $G_{\text{LNA}} = 92.8 \pm 0.04\text{dB}$ .

This leads to

$$S_E - S_{\text{off}} = G_{\text{LNA}} hf_a \sinh^2 r_E [\bar{\alpha}\gamma S_{\text{ns}} + \bar{\alpha}(1 - \gamma)S_{\text{dil},a} + \bar{\alpha}S_{\text{dil},b}] \quad (7)$$

$$S_A - S_{\text{off}} = G_{\text{LNA}} hf_a \sinh^2 r_A [\bar{\alpha}\gamma S_{\text{ns}} + (1 - \bar{\alpha}\gamma)S_{\text{dil},a} + S_{\text{dil},b}]. \quad (8)$$

Three expressions can be derived in order to calibrate the setup from these two equations.

- When the switch feeds the cold load,  $S_{\text{ns}} = S_{\text{dil},a}$  and for temperatures much smaller than a single photon  $k_B T_{\text{dil}} \ll hf_a < hf_b$ , we have  $S_{\text{ns}} = S_{\text{dil},a} = S_{\text{dil},b} = 1/2$  and from Eq. (8), we get

$$S_{\text{ns}} = S_{\text{dil},a} = \frac{1}{2} \Rightarrow G_{\text{LNA}} = \frac{S_A - S_{\text{off}}}{hf_a \sinh^2 r_A}. \quad (9)$$

- In the same conditions,

$$S_{\text{ns}} = S_{\text{dil},a} = \frac{1}{2} \Rightarrow \bar{\alpha}G_{\text{LNA}} = \frac{S_E - S_{\text{off}}}{hf_a \sinh^2 r_E}. \quad (10)$$

- The noise  $S_{\text{ns}}$  depends linearly on the load temperature  $T_{\text{ns}}$  in the high temperature limit as  $S_{\text{ns}} \sim k_B T_{\text{ns}} / hf_a$ . Therefore, the slopes of the asymptotical behaviors of the above noise differences are

$$k_B T_{\text{ns}} \gg hf_a \Rightarrow \bar{\alpha} \bar{\gamma} \mathbf{G}_{\text{LNA}} = \frac{\partial(S_E - S_{\text{off}})}{\partial k_B T_{\text{ns}}} \sinh^{-2} r_E = \frac{\partial(S_A - S_{\text{off}})}{\partial k_B T_{\text{ns}}} \sinh^{-2} r_A. \quad (11)$$

The noise power was measured according to the procedure in the table above by first ramping up (filled circles in Fig. 2) and down (open circles)  $T_{\text{ns}}$  between 10 values between 90 mK and 900 mK while keeping  $T_{\text{dil}}$  to its base value, approx. 45 mK. Each step uses a fast feedback temperature control with less than mK variations. This whole step requires about 5 hours, mainly to ensure good thermalization. The fact that up and down ramping measurement collapse is a good indication of thermalization. It is important to note that the noise measured for the nine values of the gains  $G_E$  and  $G_A$  from 3 to 100 coincide once normalized but these gains demonstrating the efficiency of the subtraction procedure used for the red and blue curves in Fig. 2.

At the end of this first step, we then switch to the cold load connected to  $T_{\text{dil}}$  and immediately perform the experiment described in the main text. We then repeat the noise power measurements for several dilution refrigerator temperature (100 mK, 180 mK, 230 mK and 260 mK) waiting 5 hours between each step to ensure again thermalization.

From the measured noise powers as a function of  $T_{\text{ns}}$  and base temperature  $T_{\text{dil}} = 45$  mK, the three relations above determine the gain  $G_{\text{LNA}} = 92.8 \pm 0.04$  dB and the losses  $\alpha = 0.33 \pm 0.05$  and  $\gamma = 0.28 \pm 0.11$  (Fig. 2). Conjugated with the fits of Fig. 3 in the main text, we get  $\beta = 0.36 \pm 0.05$ . In this experiment, the system efficiency for the coupling of the entangler to the noise source is thus  $\bar{\gamma} = 72\% \pm 11\%$ . Besides, the cross-over between zero point fluctuations and Johnson-Nyquist regimes occurs at the expected  $T_{\text{ns}}$  indicating that the cold load reaches the vacuum state.

The temperature  $T_{\text{dil}}$  of the whole setup was also varied during the experiment. It is possible to explain quantitatively the variation of noise power as a function of  $T_{\text{ns}}$  for each temperature  $T_{\text{dil}}$  with Eqs. (7) and (8) by adjusting the gain  $G_{\text{LNA}}$  with fixed  $\alpha = 0.33$  and  $\gamma = 0.28$  (as shown in Fig. 3). Since 5 to 10 hours separate each measurement at a given temperature  $T_{\text{dil}}$ , due to slow thermalization, it is likely that variations of the gain  $G_{\text{LNA}}$  are entirely due to drifts of the following amplifiers. The agreement between measurement and theoretical expectations for all temperatures and gains  $G_E$ ,  $G_A$  (Fig. 3) is then consistent with vacuum state at the input of the mixers at the lowest temperatures reported in the main text. Note that this agreement is all the more impressive that  $S_{\text{dil},a}$  and  $S_{\text{dil},b}$  do not depend identically on temperature.

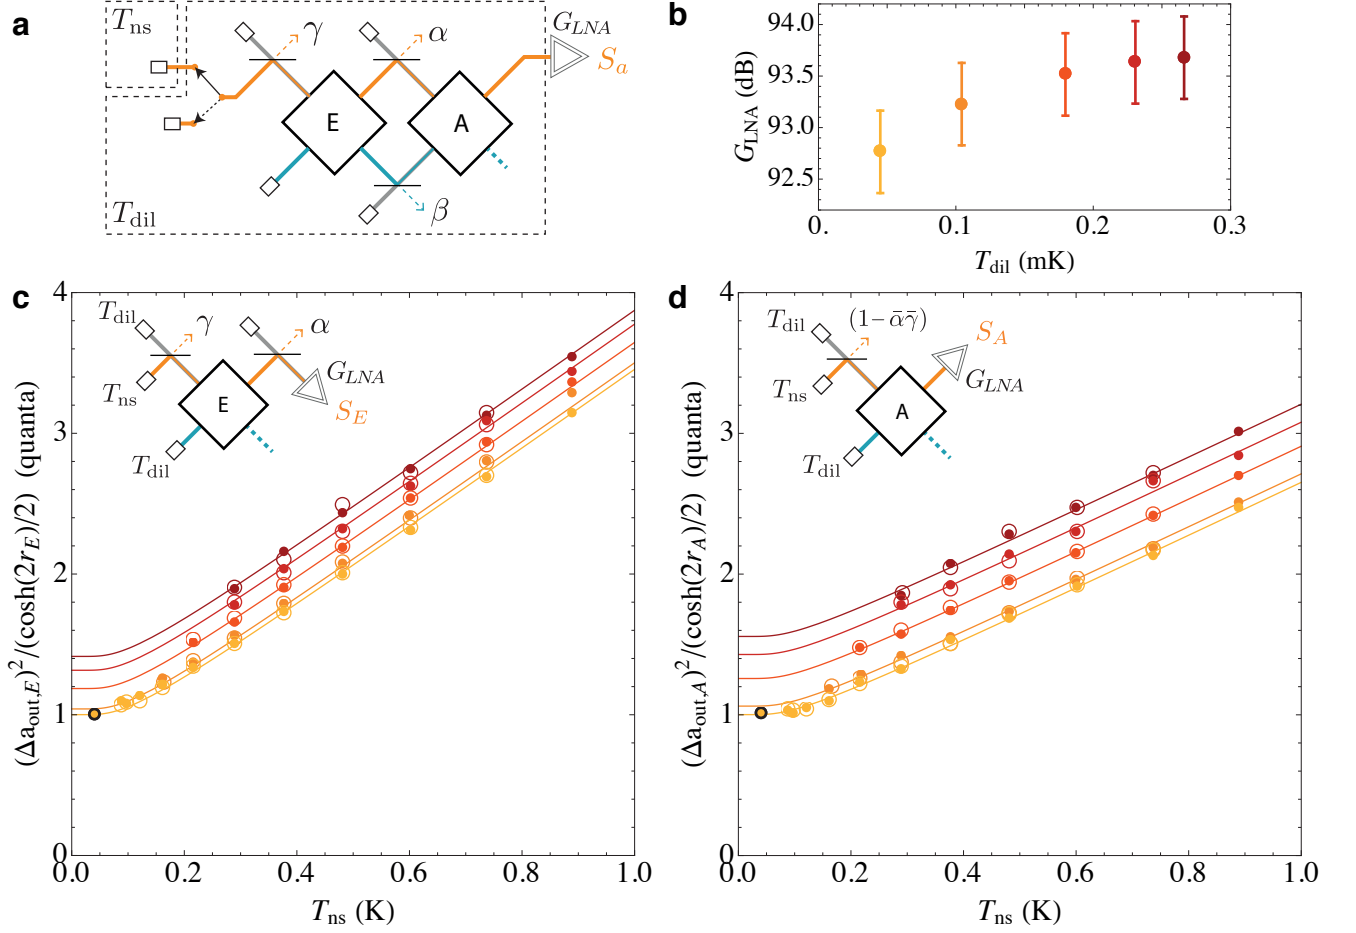

FIG. 3: **a.** Scheme of the measurement setup. **b.** Dots and error bars represent the result of the following fitting procedure. For each temperature  $T_{\text{dil}}$ , the noise measurements as a function of  $T_{\text{ns}}$ , for  $G_A = 10$  or  $G_E = 10$ , are compared to Eqs. (7,8) as in Fig. 2. The losses are fixed for all temperatures to the previously found values  $\alpha = 0.33$  and  $\gamma = 0.28$  and the gain  $G_{\text{LNA}}$  is fitted for each value of  $T_{\text{dil}}$  (single value explaining all probed values of  $T_{\text{ns}}$  for both mixers). **c.** Dots: Normalized variance of the output field, averaged over all gains  $G_E$  and  $G_A$ , obtained using Eq. (3) with the measured values of  $S_E - S_{\text{off}}$  and the fitted gain  $G_{\text{LNA}}$  from panel 3b as a function of temperature  $T_{\text{ns}}$  for various values of  $T_{\text{dil}} = 45$  mK, 100 mK, 180 mK, 230 mK and 260 mK (represented by colors from yellow to red). Circles: same data for decreasing temperatures  $T_{\text{ns}}$  from one point to the next. Lines: theory using Eq. (7) with the fit parameters from panel 3b. **d.** Same as panel 3c with the analyzer on and the entangler off. Lines use Eq. (8).

### Estimating error bars on the calibration

We estimate from Fig. 3b the value of the gain  $G_{\text{LNA}}$  used in the experiment to possibly drift by at most  $\pm 5\%$  during the measurements reported in the main text. Taking into account the standard deviation of the fitting procedure presented above, the actual uncertainty on the gain  $G_{\text{LNA}}$  used in the main text is  $\pm 10\%$ .

The relative statistical uncertainty on the measured noise spectral density  $S_a - S_{\text{off}}$  is  $\pm 1\%$ . Using the calibration formula (3), the uncertainty on the noise  $\sigma^2$  reported in the main text can be calculated and reads

$$\frac{\Delta\sigma^2}{\sigma^2} = \sqrt{(1 - 1/\sigma^2)^2 \cosh^{-2}(2r_A)(20\%)^2 + (1 + (\sigma^2)^{-2})(2\%)^2}. \quad (12)$$

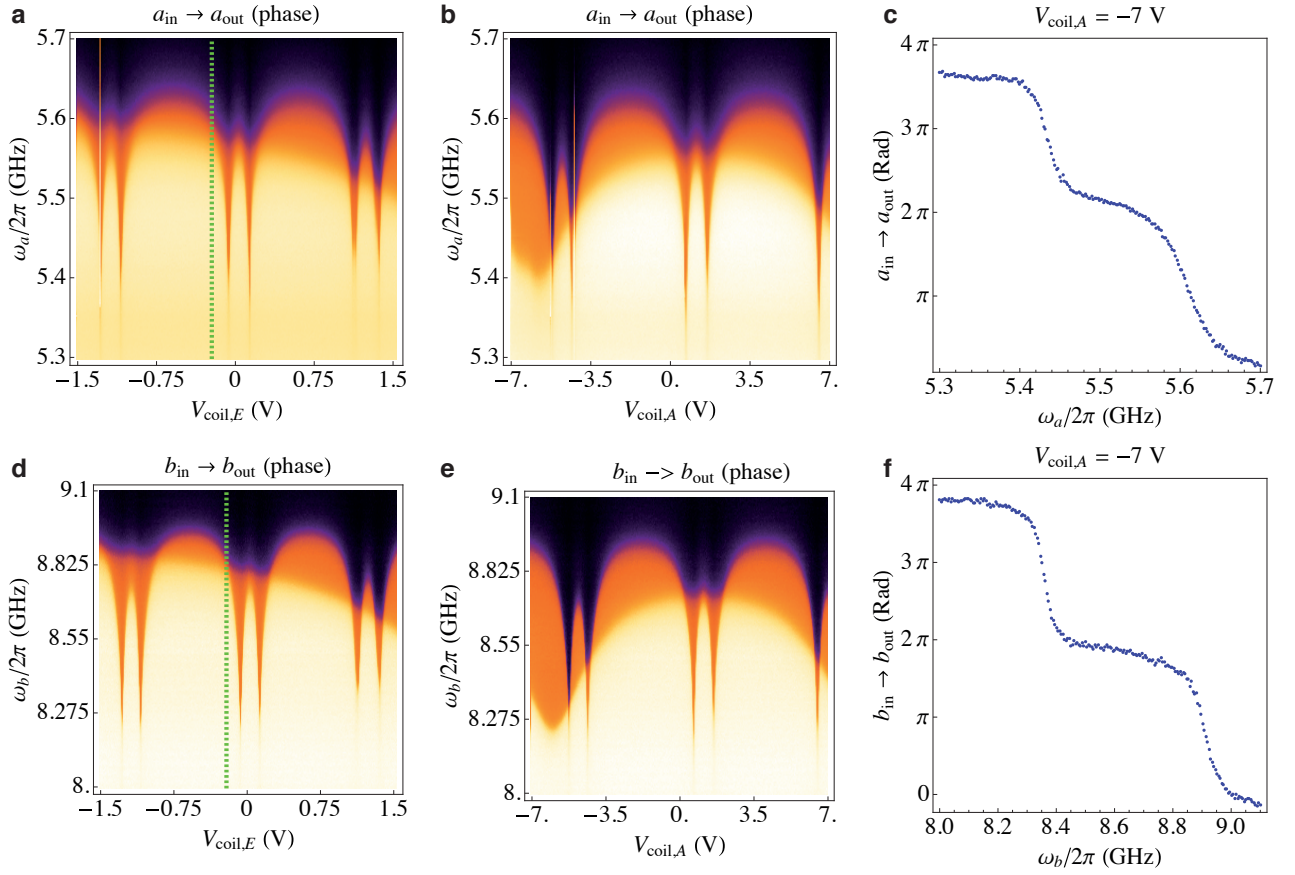

FIG. 4: **a.** Color plot representing the measured phase of the signal transmitted between  $a$  input and output ports as a function of frequency and magnetic field on the entangler. The magnetic field on the entangler is proportional to the voltage  $V_{\text{coil},E}$  across the circuit biasing the superconducting coil. No voltage  $V_{\text{coil},A}$  is applied on the coil biasing the analyzer. No pump power is applied to both mixers. The color code can be deduced from Fig. c. The green dashed line represents the experimental working point, where the measurements from the main text, have been performed. **b.** Same measurement with  $V_{\text{coil},E} = 0$  and varying  $V_{\text{coil},A}$ . **c.** Cut through the color plot b at  $V_{\text{coil},A} = -7$  V. **d.e.f.** Same measurements as above but between  $b$  input and output ports.

## CHARACTERIZATION OF THE MIXERS

As explained in Ref. [1], the resonance frequency of both modes  $a$  and  $b$  can be tuned using a magnetic field. In order to characterize the resonance frequencies, one follows the modulation of the  $2\pi$  phase shift in the measured phase of the reflected signal as a function of frequency on each port (Fig. 4). The fact that both mixers are in series implies the observation of two  $2\pi$  phase shifts. In the experiment, both mixers were located back-to-back with one magnetic coil close-by. Therefore, the main effect of changing the entangler (resp. analyzer) coil current is to tune the entangler (resp. analyzer) resonance frequencies, but since the other mixer is still weakly coupled to the field, the resonance frequencies of the analyzer (resp. entangler) are also slowly changing. In Fig. 4, this manifests in a fast variation of a  $2\pi$  phase shift on top of a slow one. The behavior of the resonance frequencies is similar to that of Ref. [1] so that the values of Josephson energy and central inductances must be similar. The experiment is performed where both couple of frequencies match (Fig. 4a,d), and close to a maximum of the non-linearity (see Ref. [1]). This matching is better than 1 MHz, which is much less than the bandwidth of the mixers.

# PREDICTION FOR THE COVARIANCE MATRIX

The expression of the expected covariance matrix at the various steps of the process can be calculated.

$$\mathbf{V}_{in,E} = \frac{1}{4} \begin{pmatrix} 1 & 0 & 0 & 0 \\ 0 & 1 & 0 & 0 \\ 0 & 0 & 1 & 0 \\ 0 & 0 & 0 & 1 \end{pmatrix} \Rightarrow \mathbf{V}_{out,E} = S(r_E, 0) \mathbf{V}_{in,E} S(r_E, 0)^T = \frac{1}{4} \begin{pmatrix} \cosh(2r_E) & 0 & \sinh(2r_E) & 0 \\ 0 & \cosh(2r_E) & 0 & -\sinh(2r_E) \\ \sinh(2r_E) & 0 & \cosh(2r_E) & 0 \\ 0 & -\sinh(2r_E) & 0 & \cosh(2r_E) \end{pmatrix} \quad (13)$$

and after the introduction of losses  $\alpha$  on both beams

$$\mathbf{V}_{in,A} = (1 - \alpha) \mathbf{V}_{out,E} + \frac{\alpha}{4} \mathbb{I}_4 = \frac{1 - \alpha}{4} \begin{pmatrix} \cosh(2r_E) + \frac{\alpha}{1-\alpha} & 0 & \sinh(2r_E) & 0 \\ 0 & \cosh(2r_E) + \frac{\alpha}{1-\alpha} & 0 & -\sinh(2r_E) \\ \sinh(2r_E) & 0 & \cosh(2r_E) + \frac{\alpha}{1-\alpha} & 0 \\ 0 & -\sinh(2r_E) & 0 & \cosh(2r_E) + \frac{\alpha}{1-\alpha} \end{pmatrix}. \quad (14)$$

The criterion for finite entanglement hence reads  $1 > 4(n - k) = (1 - \alpha)e^{-2r_E} + \alpha$  which is always verified for finite squeezing and limited losses  $\alpha < 1$ .

---

\* corresponding author: benjamin.huard@ens.fr

[1] N. Roch et al., arXiv 1202.1315v1 (2012) to be published in Phys. Rev. Lett.
